# Supplementary material for: Discrete Diffusion Schr\"odinger Bridge Matching for Graph Transformation
Source: arXiv:2410.01500 source file (2025-02-28)
Supplement: Supplementary file 3 [file appendix_table_2_additional_results.tex]

\begin{table}[h!]
\caption{
PLACE HOLDER
}
\centering
% VAL, FCD, NLL, Original NLL
\resizebox{1.0\textwidth}{!}{
\begin{tabular}{lcc|ccc|ccc}
\toprule

Model
& Type
& Kernel
& Validity$(\uparrow)$
& FCD$(\downarrow)$
& NLL$(\downarrow)$
& LogP $W_1(\downarrow)$
& QED MAD$(\downarrow)$
& SAscore MAD$(\downarrow)$
\\

\midrule

% 1.038 285.513 0.161 0.145 0.611
%DDSBM Schr¨odinger Bridge 95.3 0.896 162.102 0.134 0.118 0.398
DBM
& Bridge
& Uniform
& 89.5
& 1.038
&
& 0.161
& 0.145
& 0.611
\\

DDSBM
& Schrödinger Bridge
& Uniform
& 95.3
& 0.896
&
& 0.134
& 0.118
& 0.398
\\

\midrule

DBM
& Bridge
& Marginal
& 88.9
& 1.429
&
& 0.141
& 0.127
& 0.631
\\

DDSBM
& Schrödinger Bridge
& Marginal
& 95.6
& 0.757
&
& 0.100
& 0.113
& 0.415
\\

\bottomrule
\end{tabular}
}
\label{tab:appendix_table_3}
\end{table}
